# Supplementary material for: Language-Driven 6-DoF Grasp Detection Using Negative Prompt Guidance
Source: arXiv:2407.13842 source file (2024-07-25)
Supplement: Supplementary file 1 [file summary.tex]

\section*{Summary}
This Supplementary Material provides additional material for our paper titled \textit{``Language-Driven 6-DoF Grasp Detection Using Negative Prompt Guidance''}. The material is organized as follows:
\begin{itemize}
    \item Section~\ref{Sec: Theory} provides mathematical proof for our theory in the main paper and recalls the connection between diffusion and energy-based models.
    \item Section~\ref{Sec: Rw} provides a detailed discussion of related literature, including diffusion models in robotics and language-driven grasp detection.
    \item Section~\ref{Sec: Stats} provides additional statistics of our dataset and comparisons to others.
    \item Section~\ref{Sec: Impl} presents the implementation details of our method and other baselines.
    \item Section~\ref{Sec: abl} provides ablation studies.
    \item Section~\ref{Sec: Qual} shows additional qualitative results of our method.
    \item Section~\ref{Sec: Robot} provides additional information about our robotic experiments.
\end{itemize}
